# Supplementary material for: GaussianAvatar-Editor: Photorealistic Animatable Gaussian Head Avatar Editor
Source: arXiv:2501.09978 source file (2025-01-17)
Supplement: Supplementary file 1 [file X_suppl.tex]

\clearpage
\setcounter{page}{1}
\maketitlesupplementary

\section{Qualitative Results Gallery}
For better visualization, we refer the reader to the video in the supplementary, including:

\textbf{Our results.} We provide more qualitative results in the video, including: 
\begin{itemize}
\item Different edit prompts, shows edited results of different text prompts of the same avatar;
\item Different avatars, shows edited results of the same text prompt of different avatars; 
\item Novel view, shows novel view rendering results of edited avatars; 
\item Novel pose, that animate the edited avatars using the source actor's video.
\end{itemize}

\textbf{Our ablation studies.} To make our GaussianAvatar-Editor self-contained, we also provide qualitative results to our ablation studies WABE in the video. 

\textbf{Comparisons with baselines.} We provide more qualitative results with baselines from three takes in the video, including novel view rendering, self-reenactment, and cross-identy reenactment.
